# Supplementary material for: Noisy Submodular Maximization via Adaptive Sampling with Applications to Crowdsourced Image Collection Summarization
Source: arXiv:1511.07211 source file (2015-12-01)
Supplement: Supplementary file 1 [file appendix_experiments_feature_selection.tex]

%!TEX root = nips-bestsubselect.tex

\section{Additional Experiments --- Feature Selection}
\label{app.feat_sel}

In this section we provide additional experiments for feature selection. We first describe the task in more detail and then present our experimental results.

\subsection{Objective} 
For this task we used the \emph{Caltech-UCSD Birds-200-2011} image dataset with photos of 200 bird species~\cite{WahCUB_200_2011}.
Each image in this dataset was annotated with 312 binary attributes, e.g.\ \emph{has\_forehead\_color:red}, through workers on MTurk. Features can take values in \{+1, -1 \} indicating the presence or absence of an attribute.
We considered a binary classification task of endandegred vs. non-endagnered woodpeckers, cf.\ Figure~\ref{fig.resuts1_fs}(b).  A similar setting was considered in~\cite{singla14crowdteaching} in the context of crowdsourcing experimentation.
% $[2013-cvpr_DengKrauseFei-Fei_fine-grained-crowdsourcing]$ used the same dataset to elicit features by designing a visual game.
We reduced the 312 features to a total of 10 features as follows: We took the 3 most informative features according to a binary naive-Bayes model for classification. Additionally, we selected 3 features that were redundant to the already selected ones, e.g.\ \emph{has\_forehead\_color:red} and \emph{has\_forehead\_color:black}. We randomly sampled the remaining 4 other features. 

From these features we built a naive-Bayes classifier and used the corresponding information gain as the submodular function for our experiments.

\subsection{Results via Simulations}

Our results for the synthetic experiments for feature selection are shown in Figure~\ref{fig.resuts1_fs}. 
In our first experiment, we compare the quality of solutions obtained by algorithm $\textsc{SubmSelX}^P$ to solutions of the greedy algorithm. The utility of the sets selected during execution of the algorithm are shown in Figure~\ref{fig.resuts1_fs}(a). The results are qualitatively the same as for the image collection summarization task, as reported earlier. Here, we also computed the classification accuracy as  metric of real interest for real, cf.\ Figure~\ref{fig.resuts1_fs}(c).

%%%%%%%%%%%%%%%%%%%%%%%%%%%%%%%%%%%%%%%%%%%%%%%%%%%%%%%%%
\begin{figure*}[t!]
\centering
   \subfigure[Information gain]{
     \includegraphics[width=0.31\textwidth]{fig/results_FeatureSel_syn1.pdf}
     \label{fig.resuts1.syn2}
   }
   \subfigure[Species]{
     \includegraphics[width=0.31\textwidth]{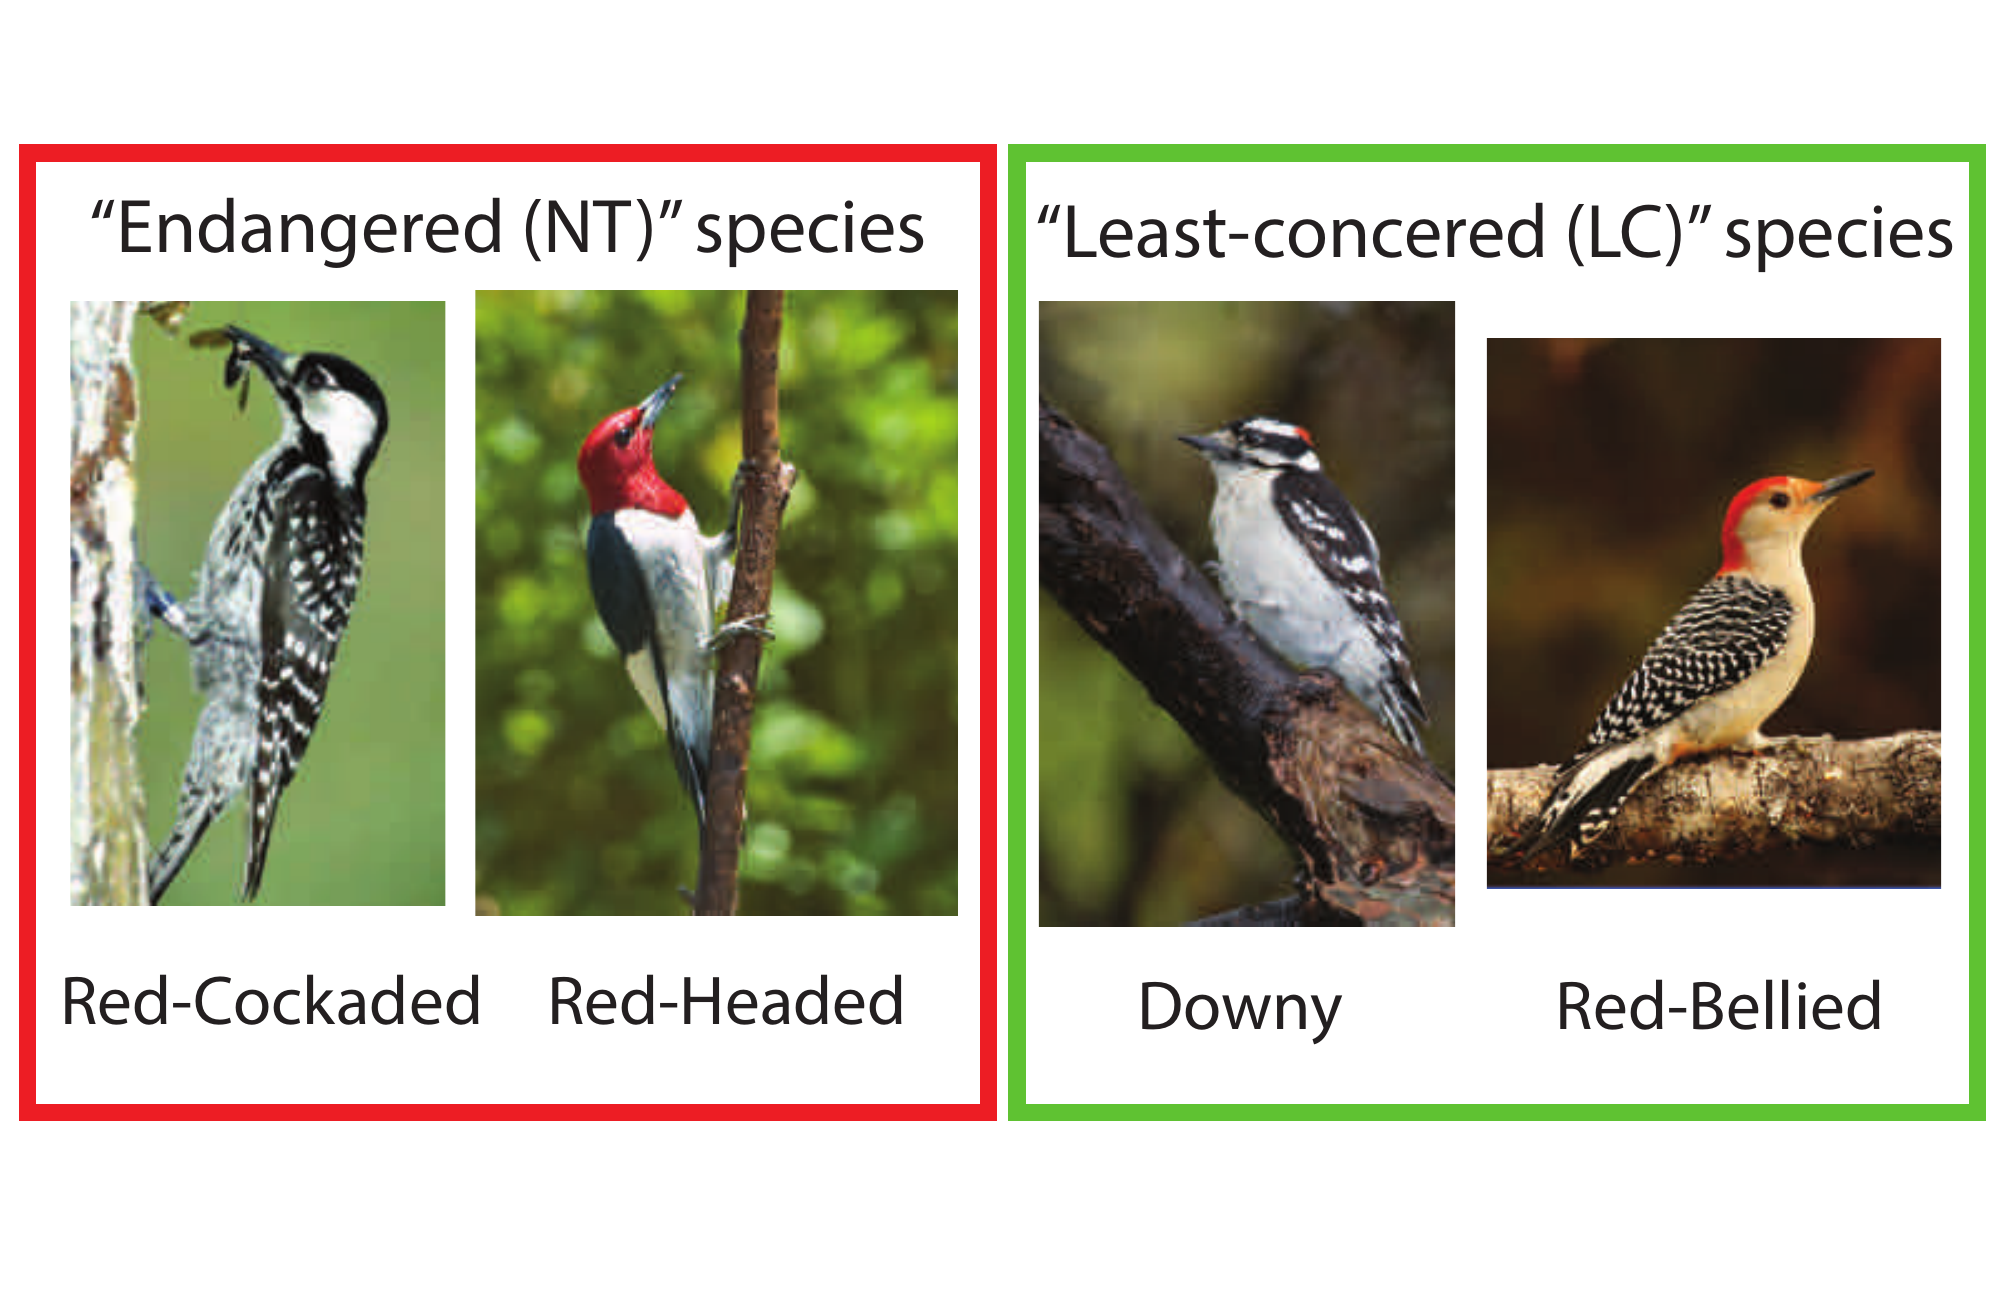}
     \label{fig.resuts1.syn1}
   }   
   \subfigure[Classification accuracy]{
     \includegraphics[width=0.31\textwidth]{fig/results_FeatureSel_syn2.pdf}
    \label{fig.resuts1.syn3}
   }
\caption{Results from synthetic simulations for feature selection.} 
\label{fig.resuts1_fs}
\end{figure*}

%%%%%%%%%%%%%%%%%%%%%%%%%%%%%%%%%%%%%%%%%%%%%%%%%%%%%%%%%
